# Supplementary material for: Pre-training Tasks for Embedding-based Large-scale Retrieval
Source: arXiv:2002.03932 source file (2020-02-10)
Supplement: Supplementary file 1 [file appendix.tex]

\section{Appendix}
You may include other additional sections here.
